# Supplementary material for: Learning Regularized Positional Encoding for Molecular Prediction
Source: arXiv:2211.12773 source file (2022-11-23)
Supplement: Supplementary file 1 [file appendix.tex]

\section{Sizing the Embedding}

\label{sec:sizing}

\begin{figure}[h]
    \centering
    \includegraphics[width=0.45\textwidth]{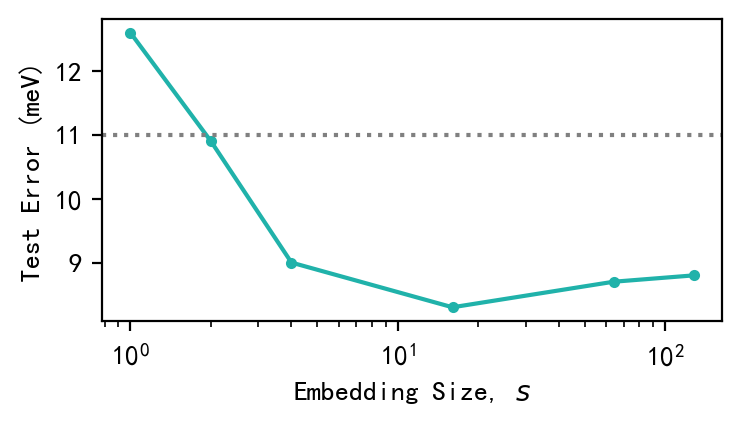}
    % \caption{The dependence of test loss on embedding size, tested on QM9 $U_0$ prediction task with EGNN as the backbone model}
    \includegraphics[width=0.35\textwidth]{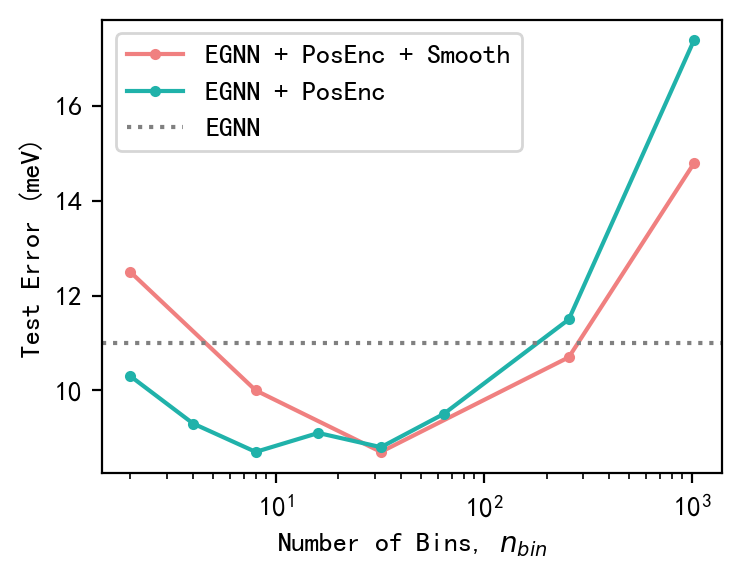}
    \caption{Left: Dependence of test loss on embedding size, tested on QM9 $U_0$ prediction task with EGNN as the backbone model. Right: Dependence of test loss on number of bins, tested on QM9 $U_0$ prediction task with EGNN as the backbone model.}
    \label{fig:emb_size}
\end{figure}

The number of bins, $n_\text{bin}$, and the embedding size $s$ are the two hyperparameters that determine the size of the embedding. They affect the accuracy of the proposed method.

As illustrated in the left panel of Figure~\ref{fig:emb_size}, the loss is large with a small embedding size. Small embedding size limits the ability of the embedding to express multi-modal nonlinearity. As the embedding size increases, the test error decreases. This indicates multiple nonlinear transformations are necessary for the model to accurately predict the labels. As the embedding size further increases, the test error no longer improves.
For the number of bins, there is a stronger non-monotonic relation between the test error and $n_\text{bin}$, as shown in the right panel of Figure~\ref{fig:emb_size}.
At a small $n_\text{bin}$, the bins are too sparse and cannot express a complex nonlinear function. This causes large loss. Adding regularization further reduce the flexibility of the embedding and increases the loss.
At a large $n_\text{bin}$, the space between bins is too small, and some bins may be never trained during training. Therefore the test loss is large with these un-trained parameters. Adding the regularization helps the bins to remain smooth, so even if a bin is not trained directly, its embedding is updated due to the changes propagated from its adjacent bins. This reduces the effects of the untrained parameters issue, and reduces the loss compared to the case without regularization.
